# Supplementary material for: The More You See in 2D, the More You Perceive in 3D
Source: arXiv:2404.03652 source file (2024-04-04)
Supplement: Supplementary file 1 [file appendix.tex]

\newpage
\appendix
\section{Appendix}

\begin{table*}[h!]
\small
    \centering
    \begin{tabular}{ccc|ccc|ccccc}
            Cam. init. & Adaptation &3D rec. losses& LPIPS& PSNR &  SSIM&  CD&  F1@0.04&  F1@0.05& F1@0.06 &VolumeIoU\\
         \toprule
            RP++&&data + SDS& 0.22 & 13.9 & 0.82 & 0.229 & 0.441 & 0.507 & 0.561 & 0.410 \\
         \midrule
            RP++*&&data + SDS& 0.17 & 17.1 & 0.85 & 0.029 & 0.872 & 0.915 & 0.944 & 0.601 \\
            RP++*&\cmark &data + SDS& 0.16 & 18.1 & 0.86 &  0.015 & 0.941 & 0.964 & 0.975 & 0.628 \\
            RP++*&\cmark &data only& 0.51 & 9.8 & 0.57 & 0.281 & 0.335 & 0.396 & 0.450 & 0.220 \\
            RP++*&\cmark &SDS only& 0.20 & 15.3 & 0.84 & 0.030 & 0.762 & 0.822 & 0.864 & 0.516 \\
    \end{tabular}
    \caption{\small \textbf{\ApproachName~ablations for 3D reconstruction.} We evaluated on 13 objects as InstantNGP failed to converge when camera poses were initialized with RP++ for 7 objects.}
    \label{tab:abl_3D_sup}
\end{table*}

You may include other additional sections here.

\begin{table*}[h!]
\centering
\begin{tabular}{l|cccc} 
\toprule
 & $\Delta$ Rot $\downarrow$ &$\Delta$ Trans $\downarrow$   & $\Delta$ az $\downarrow$&$\Delta$ el $\downarrow$\\ 
\midrule
RP++  & 96.61 & 2.97 & 80.77 & 11.52 \\
\ApproachName~w/o adaption &49.59 & 0.03 &35.01 &7.96 \\
\ApproachName  &  20.69 &- &18.47 &4.17 \\
\bottomrule
\end{tabular}
\caption{\textbf{Camera Pose Evaluation.} Errors in estimated camera rotations (in degrees) and translations (in \sg{how? normalized?}) \xinyang{In zero123, they rendered the images using radius length within a fixed range -- [1.5, 2.2], we followed this setting during rendering training set. So all the numbers are among this scale without normalizing.} using 3 input images on the Objaverse and GSO datasets. We compare the original RelPose++ trained on Co3D to our version scaled on Objaverse, and the effect of fine-tuning using \ApproachName. \sg{How is the evaluation done on Objaverse? How many images are used?}} \xinyang{We kept a subset of objaverse as testing set(100 objects) to do the pose validation.} \xinyang{21 objects}
\label{tab:left}
\end{table*}

\begin{table*}[h!]
    \centering
    \begin{tabular}{c|ccc|ccccc|c}
         \#Images&  LPIPS $\downarrow$ &  PSNR $\uparrow$ &  SSIM $\uparrow$ &  CD $\downarrow$&  F1@0.04 $\uparrow$ &  F1@0.05 $\uparrow$& F1@0.06 $\uparrow$  &VolumeIoU $\uparrow$ &Cam Rot $\downarrow$\\
         \toprule
         1 (Zero123)& 0.23 & 14.1 & 0.86 & 0.168 & 0.34 & 0.40 & 0.46 & 0.25 & - \\
         \midrule
         2& 0.13 & 18.8 & 0.88 & 0.025 & 0.87 & 0.92 & 0.95 & 0.59 & 31.94 \\
         3& 0.12 & 19.3 & 0.89 & 0.016 & 0.94 & 0.97 & 0.98 & 0.64 & 20.69 \\
         4& 0.11 & 19.7 & 0.90 & 0.014 & 0.97 & 0.99 & 0.99 & 0.73 & 8.84 \\
         5& 0.11 & 19.8 & 0.90 & 0.013 & 0.97 & 0.99 & 0.99 & 0.73 & 6.58 \\
         % 6&  &  &  &  &  &  &  & & \\
         \bottomrule
    \end{tabular}
    \caption{Backup for F1's.} 
    %Evaluating 3D reconstructions on 16 objects from the GSO dataset. Observe that both appearance and geometry improve with more views. Zero1-to-3 is the SoTA single-image approach. \sg{Will convert to a line-plot once numbers arrive.}}  \xinyang{We changed the threshold for F1-score to a suitable scale based on experiments.} \sg{Please compute numbers for F1@0.01,0.02,0.03 also.} \Xinyang{23 objects}
    \label{tab:more_img_3D_backup}
\end{table*}

\begin{table*}[h!]
\centering
\begin{tabular}{l|cc|cc|llll} 
\toprule
\multicolumn{1}{c|}{\multirow{2}{*}{Camera Pose Estimator}} & \multicolumn{2}{c|}{Objaverse} & \multicolumn{2}{c}{GSO (full)} &        \multicolumn{4}{c}{GSO (subset)}\\
\multicolumn{1}{c|}{}                                   & $\Delta$ Rot $\downarrow$ & $\Delta$ Trans $\downarrow$ & $\Delta$ Rot $\downarrow$ & $\Delta$ Trans $\downarrow$  & $\Delta$ Rot $\downarrow$ &$\Delta$ Trans $\downarrow$   & $\Delta$ az $\downarrow$&$\Delta$ el $\downarrow$\\ 
\midrule
RP++ (Co3D)       & 101.9          & 8.27          & 96.5          & 4.69           & 96.61          & 2.97 & 80.77 & 11.52 \\
RP++* (Objaverse) & 57.8 & 0.07 & \textbf{30.7} & \textbf{0.02}  &\textbf{49.59} & \textbf{0.03} &35.01 &7.96 \\
\hspace{1em} + \ApproachName-FT      & -              & -             &             -&              -& 20.69 &- &18.47 &4.17 \\
\bottomrule
\end{tabular}
\caption{\textbf{Camera Pose Evaluation:} Errors in estimated camera rotations (in degrees) and translations (in \sg{how? normalized?}) \xinyang{In zero123, they rendered the images using radius length within a fixed range -- [1.5, 2.2], we followed this setting during rendering training set. So all the numbers are among this scale without normalizing.} using 3 input images on the Objaverse and GSO datasets. We compare the original RelPose++ trained on Co3D to our version scaled on Objaverse, and the effect of fine-tuning using \ApproachName. \sg{How is the evaluation done on Objaverse? How many images are used?}} \xinyang{We kept a subset of objaverse as testing set(100 objects) to do the pose validation.} \xinyang{21 objects} \xinyang{In the final version, do we want to use both GSO full and GSO subset, or maybe we just provide our GSO benchmark as our sampled GSO object datasets?}
\label{tab:abl_camera}
\end{table*}

\paragraph{Scaling up RelPose++} Since Zero123 takes camera poses as input, we need to get the camera poses from the unposed images to finetune Zero123. We tried to directly apply state-of-the-art sparse view camera pose estimation model Relpose++~\cite{lin2023relpose++} to get camera poses, but found out that the camera pose estimation error is quite large. 
Relpose++'s generalizability is limited because it is trained on Co3D~\cite{co3d} dataset with around 19k 3D objects. Meanwhile,  Objaverse~\cite{objaverse} is a newly released 3D dataset with around 800K diverse 3D objects, 40 times larger than Co3D. So, we scaled-up the Relpose++ model on Objaverse rendering dataset to improve the capability and generalizability of Relpose++, getting a more reasonable prediction of camera poses.

\paragraph{3D Reconstruction regularization losses}
$$ \loss_{\hat{n},1} = \mathbb{E}_{X,\delta\in\mathcal{N}(0,1)} \left\| \hat{n}(X) - \hat{n}(X+\delta) \right\|^2 $$
$$ \loss_{\hat{n},2} = \mathbb{E}_\pi \left\| \Delta \mathcal{R}^{\hat{n}}_\psi(\pi) \right\|^2 \nonumber $$
% $$$$
$$ \loss_\text{Sparse} = \mathbb{E}_\pi \left\| \mathcal{R}^\text{Mask}_\psi(\pi) \right\|_1 $$
$$ \loss_\text{Opaque} = H(\mathcal{R}^\text{Mask}_\psi(\pi)) $$
$$ \loss_\text{Reg} = \lambda_{\hat{n},1} \loss_{\hat{n},1} + \lambda_{\hat{n},2} \loss_{\hat{n},2} + \lambda_\text{Sparse} \loss_\text{Sparse} + \lambda_\text{Opaque} \loss_\text{Opaque} $$

\paragraph{Camera Pose Optimization during TTA}
\xinyang{sure! During the TTT process, we optimize the camera poses concurrently with the diffusion model. The learning rate for the camera poses, denoted as $lr_{\text{pose}}$, is set to $1000 \times lr$. After each iteration, we enforce constraints to ensure the optimized poses remain within valid ranges. Specifically, during training, the range for elevation is $[0, \pi]$, the range for radius is $[1.5, 2.2]$, and there is no explicit limit for azimuth because its cosine and sine are computed and input into the model. In}

\begin{align*}
\text{elevation} &= 
\begin{cases} 
- \text{elevation}, & \text{if elevation} < 0, \\
2\pi - \text{elevation}, & \text{if elevation} > \pi, \\
\text{elevation}, & \text{otherwise},
\end{cases} \\
\text{radius} &= \text{softmax}(\text{radius}) \cdot (\text{max\_val} - \text{min\_val}) + \text{min\_val}.
\end{align*}
\yossi{Shub, I need some help with rewriting that}

\paragraph{Figures \sg{Updated}:}
\begin{enumerate} 
    \item big figure, 3D recon: zero123 (1-img) vs ours (3-img) vs ours (5-img) on GSO (transparent bg imgs: png) \xinyang{20 objects}
    
    \item half-page, 3D recon: "ours" real-world results, any number of images. \xinyang{8 real-world}
    $/shared/xinyang/threetothreed/test_recon/threestudio/experiments_XINYANG_NEW_view_5_nerf$
    $/shared/xinyang/threetothreed/test_recon/threestudio/experiments_XINYANG_XINYANG_CAP_view_5_nerf_old$

$/shared/xinyang/threetothreed/test_recon/threestudio/experiments_XINYANG_CAP_view_1_nerf$
    
    \item 2D NVS: path: \xinyang{20 objects, no failure case.}
    
    $/shared/xinyang/threetothreed/camerabooth/experiments_nvs/GSO_demo$
    \begin{enumerate}
        \item 1-img / NA   OG / Z123
        % \item 3-img / RP++ OG / Z123
        \item 3-img / RP++ Sc / Z123-FT (Ours)
        \item 5-img / RP++ Sc / Z123-FT (Ours)
        % \xinyang{We get good results on 5 imgs maybe. Maybe we can show results using 5 imgs as it would be a harder setting.} \sg{Sure, 5 is okay too. Just get the raw renderings and numbers first for 1-5. If we want to do 6 img, can do that later.}
        % \item 6-img / RP++ Sc / Z123-FT (Ours)
    \end{enumerate}
    \item system-verification (3D): 
        \begin{enumerate}
            \item 3-img / RP++ OG / Z123 \xinyang{12 objects, 4 failure case due to OOM}
            $/shared/xinyang/threetothreed/test_recon/threestudio/experiments_GSO_demo_tab3_row1_view_3_nerf$
            \item 3-img / RP++ Sc / Z123 \xinyang{14 objects}
            $/shared/xinyang/threetothreed/test_recon/threestudio/experiments_GSO_demo_tab3_row2_view_3_nerf$
            \item 3-img / RP++ Sc / Z123-FT  (Ours)  \xinyang{23 objects}
            
            both in $/shared/xinyang/threetothreed/test_recon/threestudio/experiments_GSO_demo_view_3_nerf$
            % \item 1-img / NA OG / Z123
            % \item 1-img / NA OG / Z123-FT
            % \item 3-img / RP++ Sc / Z123-FT
            \xinyang{Original results from (b) and (c) are similar so maybe changing it into the current setting (b) that uses only one input image would be a good choice.} \sg{It's okay for the results to be similar. We can highlight minor differences. What you marked as (b) isn't a single-image setting because 3 images are used for fine-tuning.}  
        \end{enumerate}
    \item system-verification (2D): \xinyang{28-25-25 objects under each folder, no failure cases}
        \begin{enumerate} 
            \item 3-img / RP++  OG / Z123*
            % $em13 /home/xinyang/scratch/zelin_dev/threetothreed/camerabooth/log_3views_relposeorg_sc$
            $/shared/xinyang/threetothreed/camerabooth/experiments_nvs/GSO_fig5_row1$            
            \xinyang{Turns the input image to be one as original z123 cannnot use information from 3 imgs comprehensively} \sg{We can call this Z123*, which is our adaptation of Z123 that can use information from multipole images using stochastic conditioning. Comparison to 1-img Z123 can remain in the 2D NVS figure (figure in this list).} \xinyang{Got it! But does that make setting (a) and (b) look similar as they are both using stochastic conditioning? Get the results first and then we'll see}
            % \item 3-img / NA   OG / Z123 
            \item 3-img / RP++ Sc / Z123*
            $em13:/home/xinyang/scratch/zelin_dev/threetothreed/camerabooth/log_3views_zero123_sc$
            \item 3-img / RP++ Sc / Z123-FT  (Ours)
            $em13:/home/xinyang/scratch/zelin_dev/threetothreed/camerabooth/log_3views_ours_sc$
        \end{enumerate}
\end{enumerate}

\begin{table}[ht]
\centering
\caption{f1-score for reconstruction from different number of input images}
\begin{tabular}{cccc}
\hline
Num of input imgs & f1--0.01 & f1--0.02 & f1--0.03 \\
\hline
1 & 0.09 & 0.19 & 0.26 \\
2 & 0.37 & 0.66 & 0.81 \\
3 & 0.41 & 0.71 & 0.86 \\
4 & 0.46 & 0.76 & 0.90 \\
5 & 0.55 & 0.83 & 0.93 \\
\hline
\end{tabular}
\label{tab:my_label}
\end{table}

\begin{table}[ht]
\centering
\caption{3D system verification. Evaluating the effect of design choices on 3D reconstructions on 50 objects from the
GSO dataset.}
\begin{tabular}{cccc}
\hline
Setting & f1--0.01 & f1--0.02 & f1--0.03 \\
\hline
1 & 0.15 & 0.27 & 0.37 \\
2 & 0.33 & 0.62 & 0.79 \\
3 & 0.41 & 0.71 & 0.86 \\
4 & 0.06 & 0.13 & 0.18 \\
5 & 0.42 & 0.71 & 0.84 \\
\hline
\end{tabular}
\label{tab:updated_scores}
\end{table}

\begin{table*}[h]
\centering
\caption{Pose estimation accuracy before and after finetuning}
\begin{subtable}{\textwidth}
\centering
\begin{tabular}{rrrrr}
\toprule
 Num of input imgs &  Rotation Error &  ELEVATION &  AZIMUTH &  RADIUS \\
\midrule
                 2 &           33.76 &       7.25 &    27.66 &    0.00 \\
                 3 &           26.24 &       8.93 &    19.63 &    0.00 \\
                 4 &           12.10 &       6.61 &    5.83 &    0.00 \\
                 5 &           11.13 &       7.09 &    1.60 &    0.00 \\
\bottomrule
\end{tabular}
\caption{Before finetuning}
\label{tab:before}
\end{subtable}

\vspace{5mm} % Adds some space between the two subtables

\begin{subtable}{\textwidth}
\centering
\begin{tabular}{rrrrr}
\toprule
 Num of input imgs &  Rotation Error &  ELEVATION &  AZIMUTH &  RADIUS \\
\midrule
                 2 &           31.95 &      5.12 &    29.06 &    0.35 \\
                 3 &           20.69 &      4.17 &     18.47 &    0.23 \\
                 4 &            8.85 &      3.15 &     6.62 &    0.18 \\
                 5 &            6.58 &      3.32 &     3.63 &    0.14 \\
\bottomrule
\end{tabular}
\caption{After finetuning}
\label{tab:after}
\end{subtable}
\end{table*}

% WARNING: do not forget to delete the supplementary pages from your submission 
% \input{sec/X_suppl}
